# Supplementary material for: Geometrical control of active turbulence in curved topographies
Source: arXiv:1805.01455 source file (2018-05-03)
Supplement: Supplementary file 1 [file SI_2018_05_03.pdf]

# Supplementary Information for: Geometrical control of active turbulence in curved topographies

D. J. G. Pearce,[1] Perry W. Ellis,[2] Alberto Fernandez-Nieves,[2] and L. Giomi[1]

[1]*Instituut-Lorentz, Universiteit Leiden, P.O. Box 9506, 2300 RA Leiden, The Netherlands*
[2]*School of Physics, Georgia Institute of Technology, Atlanta, Georgia 30332, USA*
(Dated: May 3, 2018)

## I. VISCOUS FLOW ON CURVED SURFACES

Let be $\boldsymbol{r} = \boldsymbol{r}(x^1, x^2)$ a generic surface embedded in $\mathbb{R}^3$ and parametrized by the coordinates $(x^1, x^2)$. Furthermore, let $\boldsymbol{g}_i = \partial \boldsymbol{r}/\partial x^i$ and be a basis of covariant vectors on the tangent plane, so that $g_{ij} = \boldsymbol{g}_i \cdot \boldsymbol{g}_j$ is the surface metric tensor and $\boldsymbol{g}^i$, with $\boldsymbol{g}_i \cdot \boldsymbol{g}^j = \delta_i^j$, the associated contravariant basis. The flow of an incompressible viscous fluid of density $\rho$ and velocity $\boldsymbol{v} = v^i \boldsymbol{g}_i = v_i \boldsymbol{g}^i$ is governed by following covariant generalzation of Navier-Stokes equation:

$$\rho(\partial_t + v^k \nabla_k) v^i = \nabla_j \sigma^{ij} + f^i \ , \qquad \nabla_i v^i = 0 \ , \tag{S1}$$

where $\nabla_i$ is the covariant derivative, $f^i$ a body force and $\sigma^{ij}$ is the contravariant form of the stress tensor:

$$\sigma^{ij} = \eta(\nabla^i v^j + \nabla^j v^i) - P g^{ij} \ , \tag{S2}$$

with $P$ the pressure field. On surfaces having non-zero Gaussian curvature $K \neq 0$, a flowing area element is subject to an additional shear force, resulting from the fact that the velocity field $\boldsymbol{v}$ rotates when parallel transported along a curve. This results into the following commutation properties for the covariant derivatives of vectors and tensors:

$$[\nabla_i, \nabla_j] v_k = R^l_{kji} v_l \ , \tag{S3a}$$

$$[\nabla_i, \nabla_j] T_{kl} = R^m_{kji} T_{ml} + R^m_{lji} T_{km} \ , \tag{S3b}$$

where $[\cdot, \cdot]$ is the commutator and $R^i_{jkl}$ the mixed form of the Riemann tensor. For a surface, this can be expressed purely in terms of the Gaussian curvature and the metric tensor, namely:

$$R^i_{jkl} = K(\delta^i_k g_{jl} - g_{jk} \delta^i_l) \ , \tag{S4}$$

Contracting the $i$ and $k$ indices in Eq. (S3a) and using Eq. (S4), yields:

$$[\nabla^i, \nabla_j] v_i = K v_j \ . \tag{S5}$$

Combining Eqs. (S1), (S2) and (S5) yields:

$$\rho(\partial_t + v^k \nabla_k) v^i = \eta(\Delta_{\rm B} v^i + K v^i) - \nabla^i p + f^i \ , \qquad \nabla_i v^i = 0 \ , \tag{S6}$$

where:

$$\Delta_{\rm B} = \frac{1}{\sqrt{g}} \partial_i \left( \sqrt{g}\, g^{ij} \nabla_j \right) \ , \tag{S7}$$

is the so called Bochner or rough Laplacian.

## II. VORTICITY-STREAM FUNCTION METHOD ON CURVED SURFACES

As for more traditional two-dimensional incompressible flow, a powerful approach to solve Eqs. (S6), both numerically and analytically, consists in parametrizing the solenoidal field $\boldsymbol{v}$ in terms of a scalar vorticity function $\psi$, such that:

$$v_i = \epsilon_{ij} \nabla^j \psi \ , \tag{S8}$$

where $\epsilon_{ij}$ is the antisymmetric Levi-Civita tensor, defined as follows:

$$\epsilon_{12} = -\epsilon_{21} = \sqrt{g}\;, \qquad \epsilon_{11} = \epsilon_{22} = 0\;, \tag{S9a}$$

$$\epsilon^{12} = -\epsilon^{21} = \frac{1}{\sqrt{g}}\;, \qquad \epsilon^{11} = \epsilon^{22} = 0\;. \tag{S9b}$$

Analogously, vorticity is defined as:

$$\omega = \epsilon^{ij}\nabla_i v_j = -\Delta_{\rm LB}\psi\;, \tag{S10}$$

where:

$$\Delta_{\rm LB} = \frac{1}{\sqrt{g}}\partial_i\left(\sqrt{g}\,g^{ij}\partial_j\right)\;, \tag{S11}$$

is the Laplace-Beltrami operator. Now, using again Eqs. (S3), one can prove the following commutation rule between the covariant derivative and the rough Laplacian:

$$[\nabla_i,\Delta_{\rm B}]v_j = g_{ij}\nabla^k(Kv_k) - \nabla_j(Kv_i)\;. \tag{S12}$$

Combining this with Eqs. (S6) and (S8), yields the following equation for the vorticity $\omega$:

$$\rho\left[\partial_t\omega + \epsilon^{ij}\nabla_i\omega\nabla_j\psi\right] = \eta\left[\Delta_{\rm LB}\omega - 2\nabla^k(K\nabla_k\psi)\right] + \epsilon^{ij}\nabla_i f_j\;. \tag{S13}$$

## III. NEMATODYNAMICS ON CURVED SURFACES

The extension of the $Q$−tensor formalism on curved surfaces has been thoroughly discussed by Kralj *et al.* [25]. Here we review only some basic concept and refer the reader to Ref. [25] for details. Let then $(\boldsymbol{e}_1,\boldsymbol{e}_2)$ be an orthonormal basis on the tangent plane of the surface. If the coordinates $(x^1,x^2)$ introduced in Sec. I are orthogonal, hence $g_{12} = g_{21} = 0$, such a basis is straightforwardly constructed upon normalization of the tangent vectors $(\boldsymbol{g}_1,\boldsymbol{g}_2)$, namely: $\boldsymbol{e}_i = \boldsymbol{g}_i/|\boldsymbol{g}_i|$. In the general case, one can derive an orthonormal basis from $(\boldsymbol{g}_1,\boldsymbol{g}_2)$ using the Gram-Schmidt method or choose any specific pair of orthonormal vectors available on the surface, such as the principal curvature directions. In the $(\boldsymbol{e}_1,\boldsymbol{e}_2)$ basis one can naturally define a nematic director:

$$\boldsymbol{n} = \cos\vartheta\,\boldsymbol{e}_1 + \sin\vartheta\,\boldsymbol{e}_2\;, \tag{S14}$$

as well as a nematic tensor:

$$\begin{aligned}\boldsymbol{Q} &= \frac{S}{2}(\boldsymbol{n}\boldsymbol{n} - \boldsymbol{n}^{\perp}\boldsymbol{n}^{\perp})\;,\\ &= q(\boldsymbol{e}_1\boldsymbol{e}_1 - \boldsymbol{e}_2\boldsymbol{e}_2) + p(\boldsymbol{e}_1\boldsymbol{e}_2 + \boldsymbol{e}_2\boldsymbol{e}_1)\;,\end{aligned} \tag{S15}$$

where $\boldsymbol{n}^{\perp} = -\sin\vartheta\,\boldsymbol{e}_1 + \cos\vartheta\,\boldsymbol{e}_2$ and $S$ is the local nematic order parameter defined as:

$$S = 2\sqrt{q^2+p^2}\;, \tag{S16}$$

where:

$$q = \frac{S}{2}\cos 2\vartheta\;, \qquad p = \frac{S}{2}\sin 2\vartheta\;.$$

Alternatively, one can express $\boldsymbol{n}$ and $\boldsymbol{Q}$ in the $(\boldsymbol{g}_1,\boldsymbol{g}_2)$ basis:

$$\boldsymbol{n} = n^i\boldsymbol{g}_i\;, \qquad \boldsymbol{Q} = Q^{ij}\boldsymbol{g}_i\boldsymbol{g}_j\;,$$

where:

$$n^i = \boldsymbol{g}^i\cdot(\cos\vartheta\,\boldsymbol{e}_1 + \sin\vartheta\,\boldsymbol{e}_2)\;, \tag{S17a}$$

$$Q^{ij} = S\left(n^i n^i - \frac{1}{2}g^{ij}\right)\;. \tag{S17b}$$

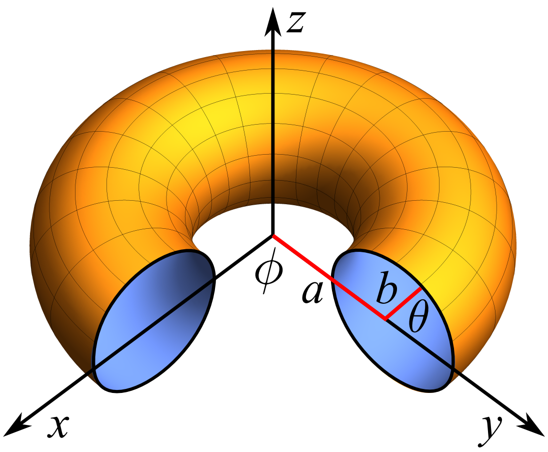


FIG. S1: Illustration of an axisymmetric torus as parameterized in Eq. (S22). The ratio $\xi = a/b$ between the radii defines the torus aspect ratio. For non-self-intersecting torii, $\xi \geq 1$.

The latter representation can be directly combined with the symmetric and antisymmetric components of the velocity gradient $\nabla \boldsymbol{v}$ to formulate a covariant version of the nematodynamic equations (see e.g. Ref. [30]). Namely:

$$(\partial_t + v^k \nabla_k) Q^{ij} = \lambda S u^{ij} + g_{kl} Q^{ik} \omega^{lj} - g_{kl} \omega^{ik} Q^{lj} + \frac{1}{\gamma} H^{ij} \;, \tag{S18}$$

where:

$$u^{ij} = \frac{1}{2} \left( \nabla^i v^j + \nabla^j v^i \right) \;, \qquad \omega^{ij} = \frac{1}{2} \left( \nabla^i v^j - \nabla^j v^i \right) \;, \tag{S19}$$

are the strain-rate and vorticity tensors, $\lambda$ is the flow-alignment parameter, $\gamma$ the rotational viscosity and $H^{ij}$ is the molecular tensor defined from the free-energy variation $\delta F = -\int \mathrm{d}A \, H^{ij} \delta Q_{ij}$. Now, as in flat space, the two-dimensional vorticity tensor has only one independent component related to the scalar vorticity defined in Eq. (S10). In particular, one can show that:

$$\omega^{ij} = \frac{1}{2} \epsilon^{ij} \omega \;, \tag{S20}$$

from which, Eq. (S18) can be cast as in Eq. (1b) of the main text. The free energy $F$ consists of a bulk term and an elastic term. Thus $F = \int \mathrm{d}A \, (f_b + f_e)$, with:

$$f_b = \frac{a_2 t}{2} Q_{ij} Q^{ij} + \frac{a_4}{4} (Q_{ij} Q^{ij})^2 \;, \tag{S21a}$$

$$f_e = \frac{k}{2} \nabla_i Q_{jk} \nabla^i Q^{jk} - \frac{k_{24}}{2} K Q_{ij} Q^{ij} + k_e Q_{ij} K^{jk} K^i_k \;, \tag{S21b}$$

where $a_2$ and $a_4$ are constants, $t$ is the reduced temperature and is negative in the nematic phase, $K_{ij} = -\boldsymbol{g}_i \cdot \partial_j N$, with $\boldsymbol{N}$ the normal vector, is the extrinsic curvature tensor and $k$, $k_{24}$ and $k_e$ are phenomenological elastic constants. The second term in Eq. (S21b) represents a two-dimensional analog of saddle-splay and $k_{24}$ could be either positive or negative. A generalization of Ericksen's inequalities imposes the constraint $-1 \leq k_{24}/k \leq 1$. The third term, first introduced in Refs. [26, 27] using the thin-film limit of a nematic shell of finite thickness, couples the nematic director with the extrinsic geometry of the surface and has the effect of aligning $\boldsymbol{n}$ along the principal direction of curvature with the least absolute principal curvature.

## IV. ACTIVE NEMATIC HYDRODYNAMICS ON THE TORUS

In this section we specify the equations given in Secs. II and III for the case of an active nematic liquid crystal confined on the axisymmetric torus. The latter is standardly parametrized in terms of the angles $\theta$ and $\phi$ marking respectively the angular distance from the $xy-$ and $xz-$plane (Fig. S1). Namely:

$$\boldsymbol{r}(\theta, \phi) = \{ (a + b\cos\theta)\cos\phi, (a + b\cos\theta)\sin\phi, b\sin\theta \} \;, \tag{S22}$$

where $a \geq b$ are respectively the large and small radius of the torus. Hereafter we will refer to as $\xi = a/b \geq 1$ to the torus aspect ratio and

$$\rho = \xi + \cos\theta \; . \tag{S23}$$

The tangent vectors along the coordinate lines are readily found:

$$\boldsymbol{g}_\theta = b\left\{-\sin\theta\cos\phi, -\sin\theta\sin\phi, \cos\theta\right\} \;, \tag{S24a}$$

$$\boldsymbol{g}_\phi = b\left\{\rho\sin\phi, \rho\cos\phi, 0\right\} \;. \tag{S24b}$$

The corresponding metric tensor is given, in covariant and contravariant from, by:

$$g_{\theta\theta} = b^2 \;, \qquad g_{\phi\phi} = b^2\rho^2 \;, \qquad g_{\theta\phi} = g_{\phi\theta} = 0 \;, \tag{S25a}$$

$$g^{\theta\theta} = \frac{1}{b^2} \;, \qquad g^{\phi\phi} = \frac{1}{b^2\rho^2} \;, \qquad g^{\theta\phi} = g^{\phi\theta} = 0 \;. \tag{S25b}$$

As on any surface of revolution, meridians ($\phi$ = const) and parallels ($\theta$ = const) of a torus are lines of principal curvature. Thus the unit vectors

$$\boldsymbol{e}_1 = \frac{\boldsymbol{g}_\theta}{|\boldsymbol{g}_\theta|} \;, \qquad \boldsymbol{e}_2 = \frac{\boldsymbol{g}_\phi}{|\boldsymbol{g}_\phi|} \;, \tag{S26}$$

identify the principal curvature directions at any point and provide a practical orthonormal basis to express the nematic director and tensor, as given by Eqs. (S14) and (S15). Their associated principal normal curvatures are given by:

$$\kappa_1 = \frac{1}{b} \;, \qquad \kappa_2 = \frac{\cos\theta}{b\rho} \;, \tag{S27}$$

whereas the corresponding geodesic curvatures given by:

$$\kappa_{g1} = 0 \;, \qquad \kappa_{g2} = \frac{\sin\theta}{b\rho} \;. \tag{S28}$$

From Eqs. (S27), the mean curvature $H$ and Gaussian curvature $H$ are readily calculated:

$$H = \frac{\xi + 2\cos\theta}{2b\rho} \;, \qquad K = \frac{\cos\theta}{b^2\rho} \;. \tag{S29}$$

The only non-zero Christoffel symbols are:

$$\Gamma^\phi_{\theta\phi} = \Gamma^\phi_{\phi\theta} = -\frac{\sin\theta}{\rho} \;, \qquad \Gamma^\theta_{\phi\phi} = \rho\,\sin\theta \;. \tag{S30}$$

Now, in the $(\boldsymbol{g}_\theta, \boldsymbol{g}_\phi)$ basis, the components of the nematic director and tensor can be expressed as follows:

$$n^\theta = \frac{\cos\vartheta}{b} \;, \qquad n^\phi = \frac{\sin\vartheta}{b\rho} \;, \tag{S31a}$$

$$Q^{\theta\theta} = \frac{q}{b^2} \;, \qquad Q^{\phi\phi} = -\frac{q}{b^2\rho^2} \;, \qquad Q^{\theta\phi} = Q^{\phi\theta} = \frac{p}{b^2\rho} \;. \tag{S31b}$$

Analogously, as shown in Ref. [35], the bulk and elastic free-energy densities, given in Eqs. (S21a) and (S21b) can be explicitly calculated in the form:

$$f_b = a_2 t(q^2 + p^2) + a_4(q^2 + p^2)^2 \;, \tag{S32a}$$

$$\begin{aligned} f_e = \frac{k}{b^2}\left\{[(\partial_\theta q)^2 + (\partial_\theta p)^2] + \frac{1}{\rho^2}[(\partial_\phi q)^2 + (\partial_\phi p)^2]\right\} + k\Psi(q^2 + p^2) \\ + \frac{4k}{b\rho}\,\kappa_{g2}\left(q\partial_\phi p - p\partial_\phi q\right) - k_{24}K(q^2 + p^2) - h_e q \;, \end{aligned} \tag{S32b}$$

where we have called introduced:

$$\Psi = H^2 - 2K + 4\kappa_{g2}^2 \,, \tag{S33a}$$

$$h_e = k_e(\kappa_2^2 - \kappa_1^2) = -k_e \frac{\xi(\xi + 2\cos\theta)}{b^2\rho^2} \,. \tag{S33b}$$

The quantity $h_e$, in particular, plays the role of an extrinsic curvature field that tends to align the nematic director along the principal direction of curvature with the least absolute principal curvature. The molecular tensor can be calculated in the basis $(\boldsymbol{e}_1, \boldsymbol{e}_2)$ using:

$$h_0 = \partial_\theta \left[\frac{\partial(\sqrt{g}\,f)}{\partial(\partial_\theta q)}\right] + \partial_\phi \left[\frac{\partial(\sqrt{g}\,f)}{\partial(\partial_\phi q)}\right] - \frac{\partial(\sqrt{g}\,f)}{\partial q} \,, \tag{S34a}$$

$$h_m = \partial_\theta \left[\frac{\partial(\sqrt{g}\,f)}{\partial(\partial_\theta p)}\right] + \partial_\phi \left[\frac{\partial(\sqrt{g}\,f)}{\partial(\partial_\phi p)}\right] - \frac{\partial(\sqrt{g}\,f)}{\partial p} \,, \tag{S34b}$$

where $\sqrt{g} = b^2\rho$ and $f = f_b + f_e$, and then expressed in the $(\boldsymbol{g}_\theta, \boldsymbol{g}_\phi)$ basis:

$$H^{\theta\theta} = \frac{h_0}{b^2} \,, \qquad H^{\theta\phi} = \frac{h_m}{b^2\rho} \,.$$

This yields:

$$\begin{aligned} H^{\theta\theta} &= -2\rho\left[a_2 t + 2a_4(q^2+p^2)\right] q - 2k\rho\Psi q + 2k_{24}\rho K q + \rho h_e \\ &+ \frac{2k\rho}{b^2}\,\partial_\theta^2 q + \frac{2k}{b^2\rho}\,\partial_\phi^2 q - \frac{2k}{b^2}\,\sin\theta\,\partial_\theta q - \frac{8k}{b}\,\kappa_{g2}\,\partial_\phi p \,, \end{aligned} \tag{S35a}$$

$$\begin{aligned} H^{\theta\phi} &= -2\left[a_2 t + 2a_4(q^2+p^2)\right] p - 2k\Psi p + \frac{2k_{24}}{b^2\rho}\,Kp \\ &+ \frac{2k}{b^2}\,\partial_\theta^2 p + \frac{2k}{b^2\rho^2}\,\partial_\phi^2 p - \frac{2k}{b^2\rho}\,\sin\theta\,\partial_\theta p + \frac{8k}{b\rho}\,\kappa_{g2}\,\partial_\phi q \,. \end{aligned} \tag{S35b}$$

In our numerical calculations we set $a_2 = 2a_4 = 2k$ and $t = 1/4$, so that, at equilibrium, $S = 1$. After further manipulation, we obtain an explicit set of equations for the components $Q^{\theta\theta}$ and $Q^{\phi\phi}$ suited to be solved numerically. Namely:

$$\partial_t Q^{\theta\theta} = \frac{\lambda S}{b^2}\,\partial_\theta v^\theta - \omega\rho\,Q^{\theta\phi} + \frac{1}{\gamma}\,H^{\theta\theta} \tag{S36a}$$

$$- v^\theta\partial_\theta Q^{\theta\theta} - v^\phi\partial_\phi Q^{\theta\theta} - 2v^\phi\sin\theta\,\rho Q^{\theta\phi}, \tag{S36b}$$

$$\partial_t Q^{\theta\phi} = \frac{\lambda S}{2b^2}\left(\partial_\theta v^\phi + \frac{\partial_\phi v^\theta}{\rho^2}\right) + \frac{\omega}{\rho}\,Q^{\theta\theta} + \frac{1}{\gamma}\,H^{\theta\phi} \tag{S36c}$$

$$- v^\theta\partial_\theta Q^{\theta\phi} - v^\phi\partial_\phi Q^{\theta\phi} + \frac{1}{\rho}\,v^\theta\sin\theta\,Q^{\theta\phi} + \frac{2}{\rho}\,v^\phi\sin\theta\,Q^{\theta\theta} \,. \tag{S36d}$$

Finally, Eqs. (S36) are coupled with Eqs. (S8), (S10) and (S13), governing the dynamics of the incompresible flow, with the body force $\boldsymbol{f} = \nabla\cdot\boldsymbol{\sigma}_{\rm a}$ set by the active stress $\boldsymbol{\sigma}_{\rm a} = \alpha\boldsymbol{Q}$. This yields:

$$\rho\partial_t\omega = \eta\left[\Delta_{\rm LB}\omega - 2\nabla^i(K\nabla_i\psi)\right] + \alpha\epsilon^{ij}\nabla_i\nabla^k Q_{jk} \,, \tag{S37}$$

where we have dropped the convective derivative on the left-hand side of Eq. (S13) to account for the fact that the Reynolds number is of order $10^{-5} - 10^{-4}$ in experiments. The last term on the right-hand side of Eq. (S37) is given explicitly by:

$$\epsilon^{ij}\nabla^k Q_{jk} = \frac{2}{\rho^2}\,\sin\theta\,\partial_\phi Q^{\theta\theta} - \frac{2}{\rho}\,\partial_{\theta\phi}^2 Q^{\theta\theta} \tag{S38}$$

$$+ \rho\,\partial_\theta^2 Q^{\theta\phi} - \frac{1}{\rho}\,\partial_\phi^2 Q^{\theta\phi} - 5\sin\theta\,\partial_\theta Q^{\theta\phi} + \left(\frac{3}{\rho}\,\sin^2\theta - 3\cos\theta\right) Q^{\theta\phi} \,. \tag{S39}$$

## V. PARTICLE MODEL OF DEFECT DYNAMICS

Here we provide an explicit derivation of the various terms in Eqs. (3) in the main text. As in the case of passive nematic defects, the forces arising from the defect-defect interaction, can be calculated starting from the Frank free-energy:

$$F_{\rm F}=\frac{1}{2}\,k\int {\rm d}A\,|\nabla\boldsymbol{n}|^2=\frac{1}{2}\,k\int {\rm d}A\,|\nabla\vartheta-\boldsymbol{A}|^2\;, \tag{S40}$$

where $A_i=\boldsymbol{e}_1\cdot\partial_i\boldsymbol{e}_2$ is the spin-connection that accounts for the rotation of the basis vectors $\boldsymbol{e}_1$ and $\boldsymbol{e}_2$ and such that $\nabla\times\boldsymbol{A}=K$ [31, 32]. If the distortion of the nematic director results solely from the defects, Eq. (S40) can be expressed into the from:

$$F_{\rm F}=\frac{1}{2}\,k\int {\rm d}A\,|\nabla\varphi|^2\;, \tag{S41}$$

where $\varphi$ is a geometric potential that given by:

$$\Delta_{\rm LB}\varphi=\rho_c-K\;, \tag{S42}$$

where $\rho_c$ is the topological charge density. For a discrete distribution of topological defects, this is given by:

$$\rho_c(\boldsymbol{r})=2\pi\sum_{n=1}^{N}s_n\delta(\boldsymbol{r}-\boldsymbol{r}_n)\;. \tag{S43}$$

The total topological charge, in turn, is constraint by the Poincaré-Hopf theorem:

$$\sum_{n=1}^{N}s_n=\chi\;, \tag{S44}$$

where $\chi$ is the Euler characteristic of the surface. For the special case of a torus $\chi=0$ and the topological charge distribution is globally neutral. Solving Eq. (S42) allows to recast Eq. (S41) as the two-dimensional Coulomb energy, namely:

$$F_{\rm F}=-4\pi^2k\sum_{n<m}s_ns_mG(\boldsymbol{r}_n,\boldsymbol{r}_m)+2\pi k\sum_{n}s_n\int {\rm d}A\,G(\boldsymbol{r}_n,\boldsymbol{r})K(\boldsymbol{r})+F_{\rm self}\;, \tag{S45}$$

where $G(\boldsymbol{r},\boldsymbol{r}')$ is the Green function of the Laplace-Beltrami operator and $F_{\rm self}$ is the self-energy resulting from the cut-off of the integral at the defect core and independent on the defect position. The first term in Eq. (S45) represents the energetic contribution associated with defect-defect interaction, whereas the second terms corresponds to the interaction between the defects and the Gaussian curvature of the substrate.

In the absence of activity, nematic disclinations can be then thought as point-like particle whose dynamics is governed by the overdamped Newton's equation:

$$\frac{{\rm d}\boldsymbol{r}_n}{{\rm d}t}=-\mu\nabla_{\boldsymbol{r}_n}F_{\rm F}\;, \tag{S46}$$

where $\mu$ is a mobility coefficient. As explained in the main text and in Refs. [4,5,36], activity drives self-propulsion of the $+1/2$ defects leading to Eq. (3a) in the main text. For an axisymmetric torus, the Laplacian Green function reads (see e.g. Ref. [31]):

$$G(\boldsymbol{r},\boldsymbol{r}')=G_0(\boldsymbol{r},\boldsymbol{r}')-\langle G_0(\boldsymbol{r},\,\cdot\,)\rangle-\langle G_0(\,\cdot\,,\boldsymbol{r}')\rangle+\langle G_0(\,\cdot\,,\,\cdot\,)\rangle\;, \tag{S47}$$

where $\langle G_0(\boldsymbol{r},\,\cdot\,)\rangle$ indicate a spatial average with respect to the dotted variable and $G_0(\boldsymbol{r},\boldsymbol{r}')$ is given by:

$$G_0(\boldsymbol{r},\boldsymbol{r}')=\frac{\log 2}{6\pi}-\frac{1}{4\pi^2\kappa}\,(\phi-\phi')^2+\frac{1}{2\pi}\,\log\left|\frac{\vartheta_1\left(\frac{z-z'}{\kappa}\,\middle|\,\frac{2i}{\kappa}\right)}{\vartheta'^{\frac{1}{3}}\left(0\,\middle|\,\frac{2i}{\kappa}\right)}\right|\;, \tag{S48}$$

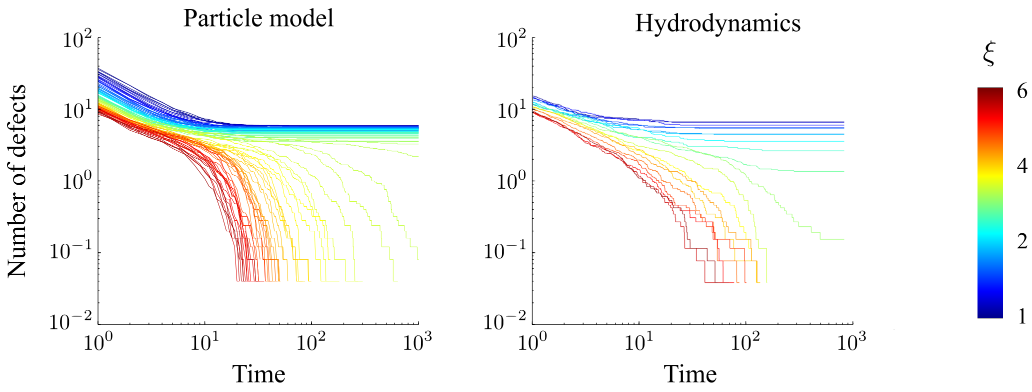


FIG. S2: Coarsening of toroidal nematics from a highly defective configuration obtained from an numerical solutions of Eq. (S52) (left) and Eqs. (1) in the main text (right). The number of defects decreases in time (expressed in terms of iterations), but, for sufficiently small aspect ratios, does not vanish. Thus "fat" tori are always populated by a finite number of defects pairs, such that the $+1/2$ defects are located along the external equator of the torus, where the Gaussian curvature is maximally positive, and $-1/2$ defects are on the internal equator, where the Gaussian curvature is maximally negative.

where:

$$z = \kappa \arctan\left(\omega \tan\frac{\theta}{2}\right) + i\phi \,, \tag{S49}$$

is a complex coordinate resulting from conformally mapping the torus onto the complex plane and we have called:

$$\kappa = \frac{2}{\sqrt{\xi^2 - 1}} \,, \qquad \omega = \sqrt{\frac{\xi - 1}{\xi + 1}} \,.$$

The function $\vartheta_1(u|\tau) = \vartheta_1(u, q)$, with $q = \exp(i\pi\tau)$, is the Jacobi theta function, defined as:

$$\vartheta_1(u, q) = 2q^{\frac{1}{4}} \sin u \prod_{n=1}^{\infty} (1 - 2q^{2n} \cos 2u + q^{4n})(1 - q^{2n}) \,. \tag{S50}$$

Finally, with these expressions in hand and upon parametrizing the direction of motion of $+1/2$ defects, by the unit vector

$$\boldsymbol{p} = \cos\psi \, \boldsymbol{e}_\theta + \sin\psi \, \boldsymbol{e}_\phi \,, \tag{S51}$$

Eqs. (3) in the main text can be explicitly written in terms of the coordinates of a single defect, namely:

$$\frac{\mathrm{d}\theta_n}{\mathrm{d}t} = \frac{1}{b}\left(v_0 \cos\psi - \frac{\mu}{b}\frac{\partial F_\mathrm{F}}{\partial \theta_n} + \zeta^t_{\theta,n}\right) \tag{S52a}$$

$$\frac{\mathrm{d}\phi_n}{\mathrm{d}t} = \frac{1}{a + b\cos\theta_n}\left(v_0 \sin\psi - \frac{\mu}{a + b\cos\theta_n}\frac{\partial F_\mathrm{F}}{\partial \phi_n} + \zeta^t_{\phi,n}\right) \tag{S52b}$$

$$\frac{\mathrm{d}\psi_n}{\mathrm{d}t} = \zeta^r_n + \frac{\mathrm{d}\phi_n}{\mathrm{d}t}\sin\theta_n \,, \tag{S52c}$$

where the derivatives of the free-energy are given by:

$$\frac{\partial F_\mathrm{F}}{\partial \theta_n} = -\frac{2}{\kappa}\sum_{m\neq n}\frac{s_n s_m}{\xi + \cos\theta_n}\,\pi\,\Re\left[\frac{\vartheta_1'}{\vartheta_1}\right]_{nm} + 2\pi s_n \frac{\sin\theta_n}{\xi + \cos\theta_n} \,, \tag{S53a}$$

$$\frac{\partial F_\mathrm{F}}{\partial \phi_n} = \frac{2}{\kappa}\sum_{m\neq n} s_n s_m \left\{(\phi_n - \phi_m) + \pi\,\Im\left[\frac{\vartheta_1'}{\vartheta_1}\right]_{nm}\right\} \,, \tag{S53b}$$

where $\Re[\,\cdot\,]$ and $\Im[\,\cdot\,]$ stand, respectively, for the real and imaginary parts and we have introduced the simplified notation:

$$\left[\frac{\vartheta_1'}{\vartheta_1}\right]_{nm} = \frac{\vartheta_1'\left(\frac{z_n-z_m}{\kappa}\,\middle|\,\frac{2i}{\kappa}\right)}{\vartheta_1\left(\frac{z_n-z_m}{\kappa}\,\middle|\,\frac{2i}{\kappa}\right)}\,.$$

## VI. COARSENING DYNAMICS OF PASSIVE TOROIDAL NEMATICS

As a benchmark problem to test the two approaches discussed in the main text and, in more detail, in Secs. IV and V, we have analyzed the coarsening dynamics of a passive toroidal nematic. The system is initalizied in a highly defective configuration and the left free to relax. In the particle model, defect annihilation is handled as explained in the main text, but annihilated defects are not reintroduced.

Fig. S2 shows a comparison between the results obtained by the particle (left) and hydrodynamic model (right). The number of defects decays in time, but plateaus to a finite value for sufficiently “fat” tori (i.e. tori with small aspect ratio), consistent with Refs. [31, 34]. The arrangement of the defects is dictated by the magnitude of the Gaussian curvature. Thus, $+1/2$ defects are located along the external equator of the torus, where the Gaussian curvature is maximally positive, and $-1/2$ defects are on the internal equator, where the Gaussian curvature is maximally negative. As for the case of active nematic tori, the two approaches used in this work are in excellent agreement with each other.
